# Supplementary material for: Low-Dimension-to-High-Dimension Generalization And Its Implications for Length Generalization
Source: arXiv:2410.08898 source file (2025-10-05)
Supplement: Supplementary file 1 [file appendix_LDHD.tex]

\section{Intuitive Illustration of LDHD Generalization}\label{appdx:ldhd}

LDHD generalization is a special scenario of OOD generalization with structural distributional shifts. The unique structure captures the inherent scaling challenge in length generalization. \cref{fig:iid-ood-ldhd} is an intuitive comparison of in-distribution, (typical) OOD generalization, and LDHD generalization.

\begin{figure}[tbhp]
    \centering
    \begin{subfigure}{0.32\linewidth}
        \centering
        \includegraphics[width=\linewidth]{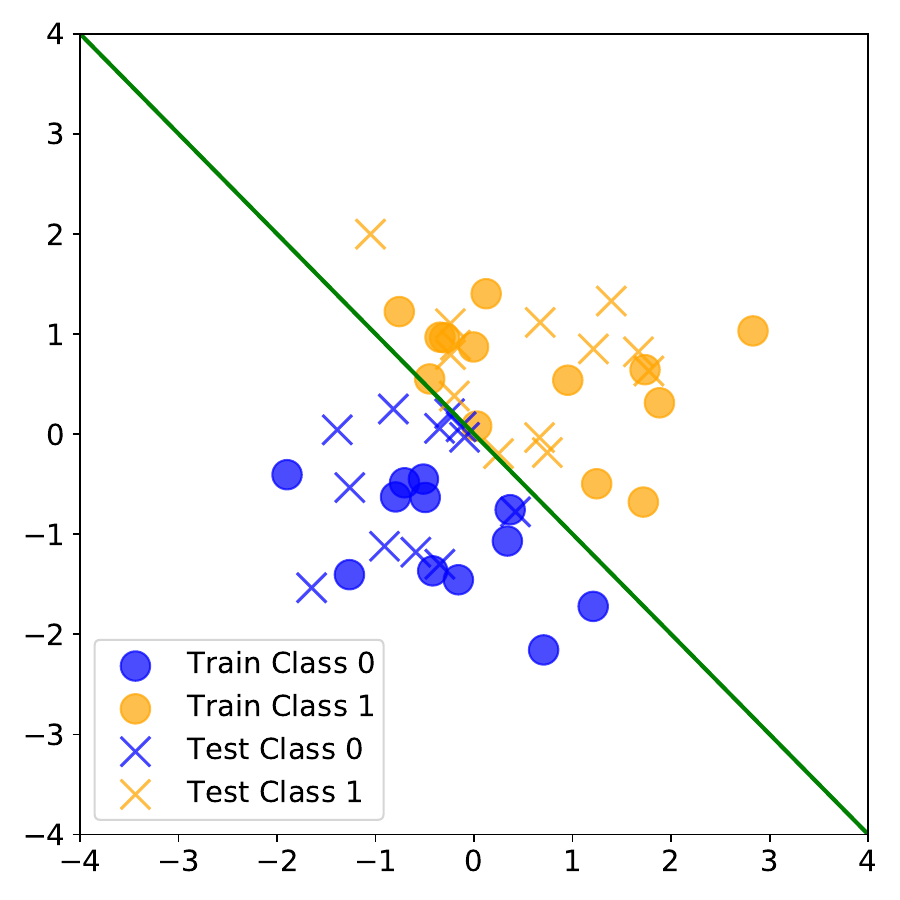}
        \subcaption{In-Distribution Generalization.}
        \label{subfig:iid}
    \end{subfigure}
    \hfill
    \begin{subfigure}{0.32\linewidth}
        \centering
        \includegraphics[width=\linewidth]{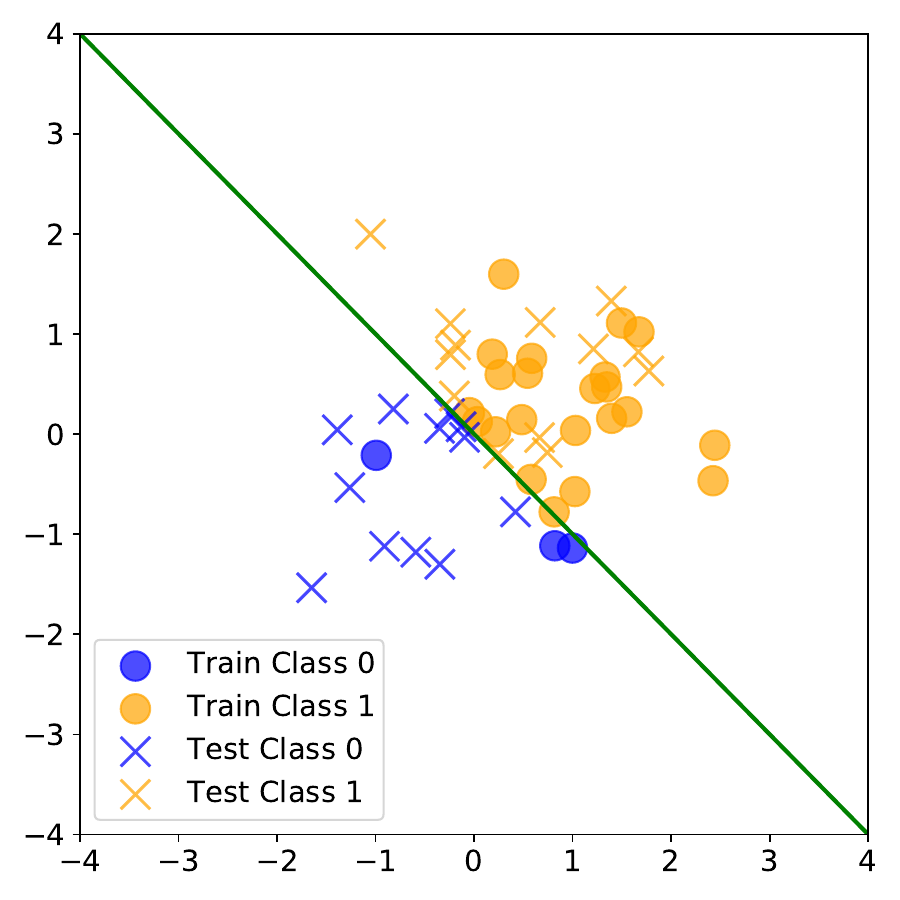}
        \subcaption{(Typical) OOD Generalization.}
        \label{subfig:ood}
    \end{subfigure}
    \hfill
    \begin{subfigure}{0.32\linewidth}
        \centering
        \includegraphics[width=\linewidth]{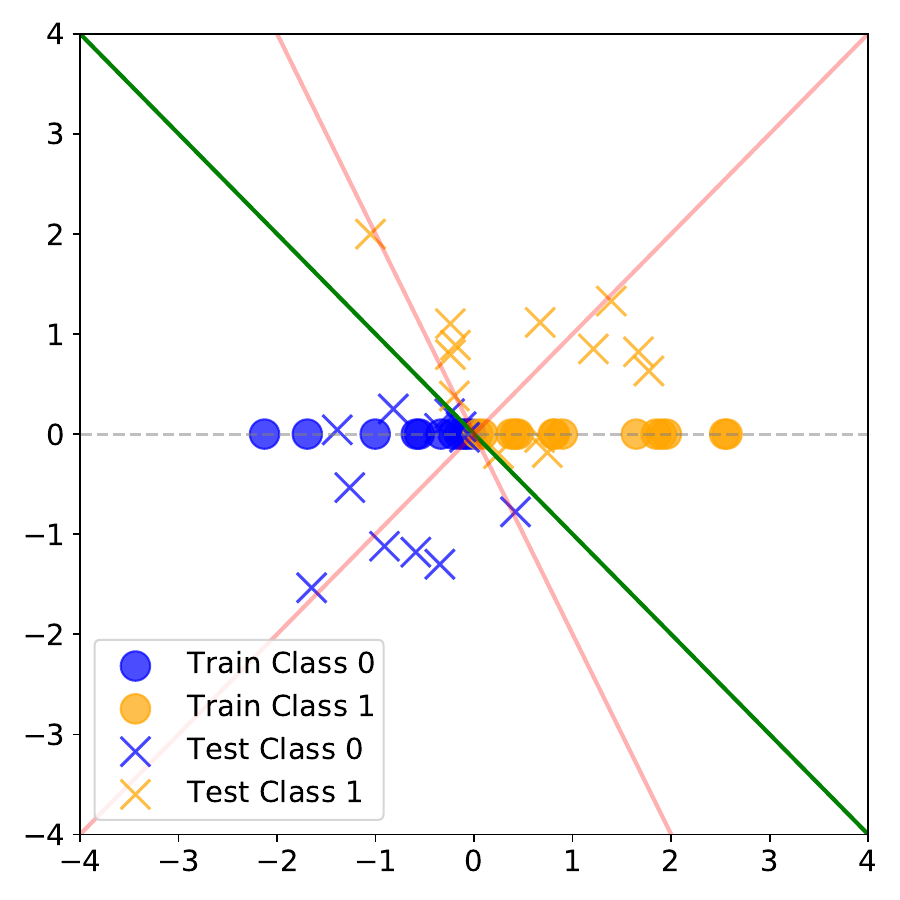}
        \subcaption{LDHD Generalization.}
        \label{subfig:ldhd}
    \end{subfigure}
    \caption{Illustrative comparison between in-distribution generalization, typical out-of-distribution generalization (with distributional shift), and LDHD generalization. (a) For in-distribution generalization, the training distribution and the testing distribution are identical. (b) For typical OOD generalization, there is a shift between the training distribution and the testing distribution. The two distributions are somewhat "close" (e.g., sharing the same support set or having a small distributional distance). (c) For LDHD generalization, the training distribution and the testing distribution can be very different. While LDHD generalization can be seen as a type of OOD generalization, the shift has a special structure from a low-dimension subspace to a higher-dimension space. This makes LDHD generalization particularly challenging because the training data reveal no information about how the extra dimension contributes to the label. For example, suppose that we are learning a linear decision boundary from the low-dimension training data. We need to know the slope of the decision boundary as a prior; otherwise we will fail to achieve LDHD generalization. 
    While all the three solid lines in (c) perfectly separate the training data, only the true decision boundary can achieve LDHD generalization.}
    \label{fig:iid-ood-ldhd}
\end{figure}
